# Supplementary material for: Think about it! Improving defeasible reasoning by first modeling the question scenario
Source: arXiv:2110.12349 source file (2021-10-24)
Supplement: Supplementary file 2 [file appendix.tex]

\appendix

\section{Appendix}
\label{sec:appendix}

\subsection{Examples of errors in the explanation structures generated by \GEN}
\squishlist
\item Figure \ref{fig:snliexample} shows an example of incorrect graph generated for Defeasible SNLI data.
\item Figure \ref{fig:socialexample} shows an example of incorrect graph generated for Defeasible Social data.
\item Figure \ref{fig:atomicexample} shows an example of incorrect graph generated for Defeasible ATOMIC data.
\squishend

\subsection{Reproducibility}
\subsubsection{\GEN, \GENS, \CORR}
T5-11B models has 11B parameters with 24-layers, 1024-hidden-state, 65,536 feed-forward hidden-state, 128 attention heads.
We use TPU (v3-8) on Google cloud platform. 
It takes 3 hours in average to train \GEN and \GENS, and 4 hours to train \CORR.

\subsubsection{Classifier for defeasible tasks}
We build on the implementation by~\citet{wolf2019huggingface}, using the default hyperparameters.
For optimization, we use AdamW~\cite{loshchilov2017decoupled} with a learning rate of 2e-5, a batch size of 16, and a linear rate scheduler with warm up for the first 3 (10\%) of the epochs.
We use accumulate gradients for two batches, and clip gradients at 1.
We also experimented with a block size of 300 and a batch size of 2.
All of our experiments were done on a single Nvidia GeForce \textsc{rtx} 2080 Ti.


\begin{figure*}
\centering
\begin{minipage}{.5\textwidth}
  \centering
  \includegraphics[width=.8\linewidth]{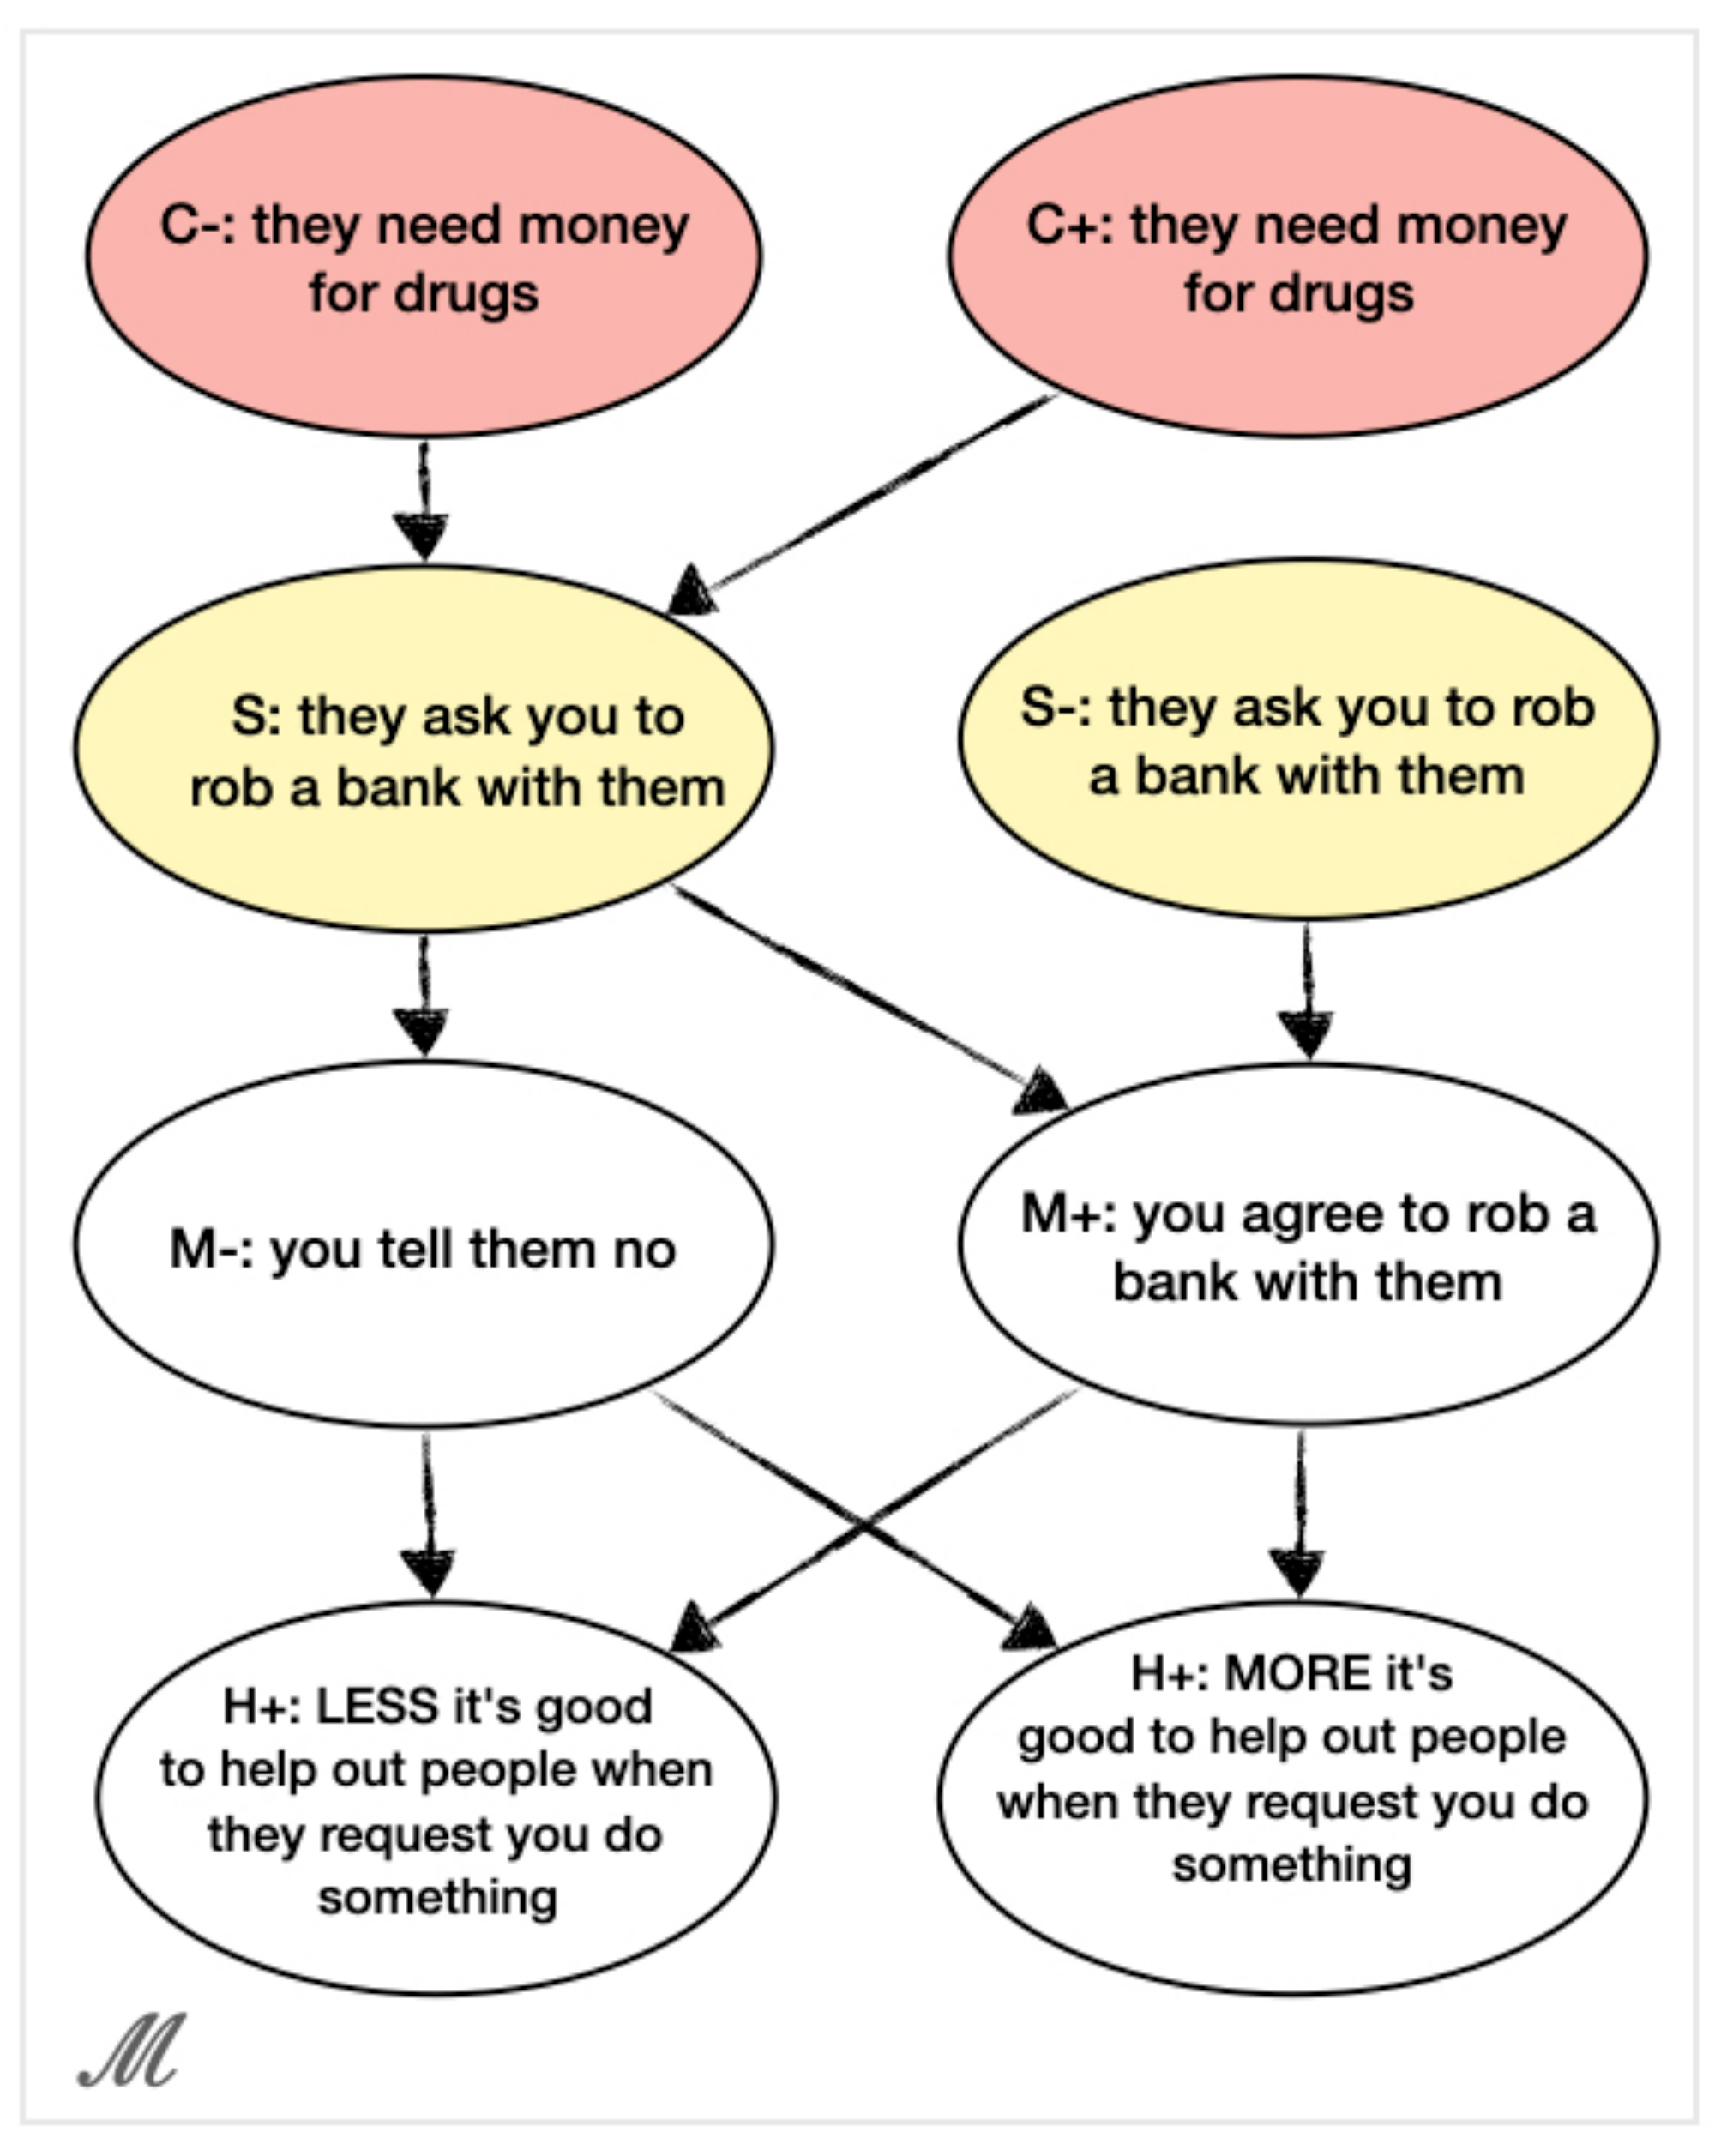}
\end{minipage}%
\begin{minipage}{.5\textwidth}
  \centering
  \includegraphics[width=.8\linewidth]{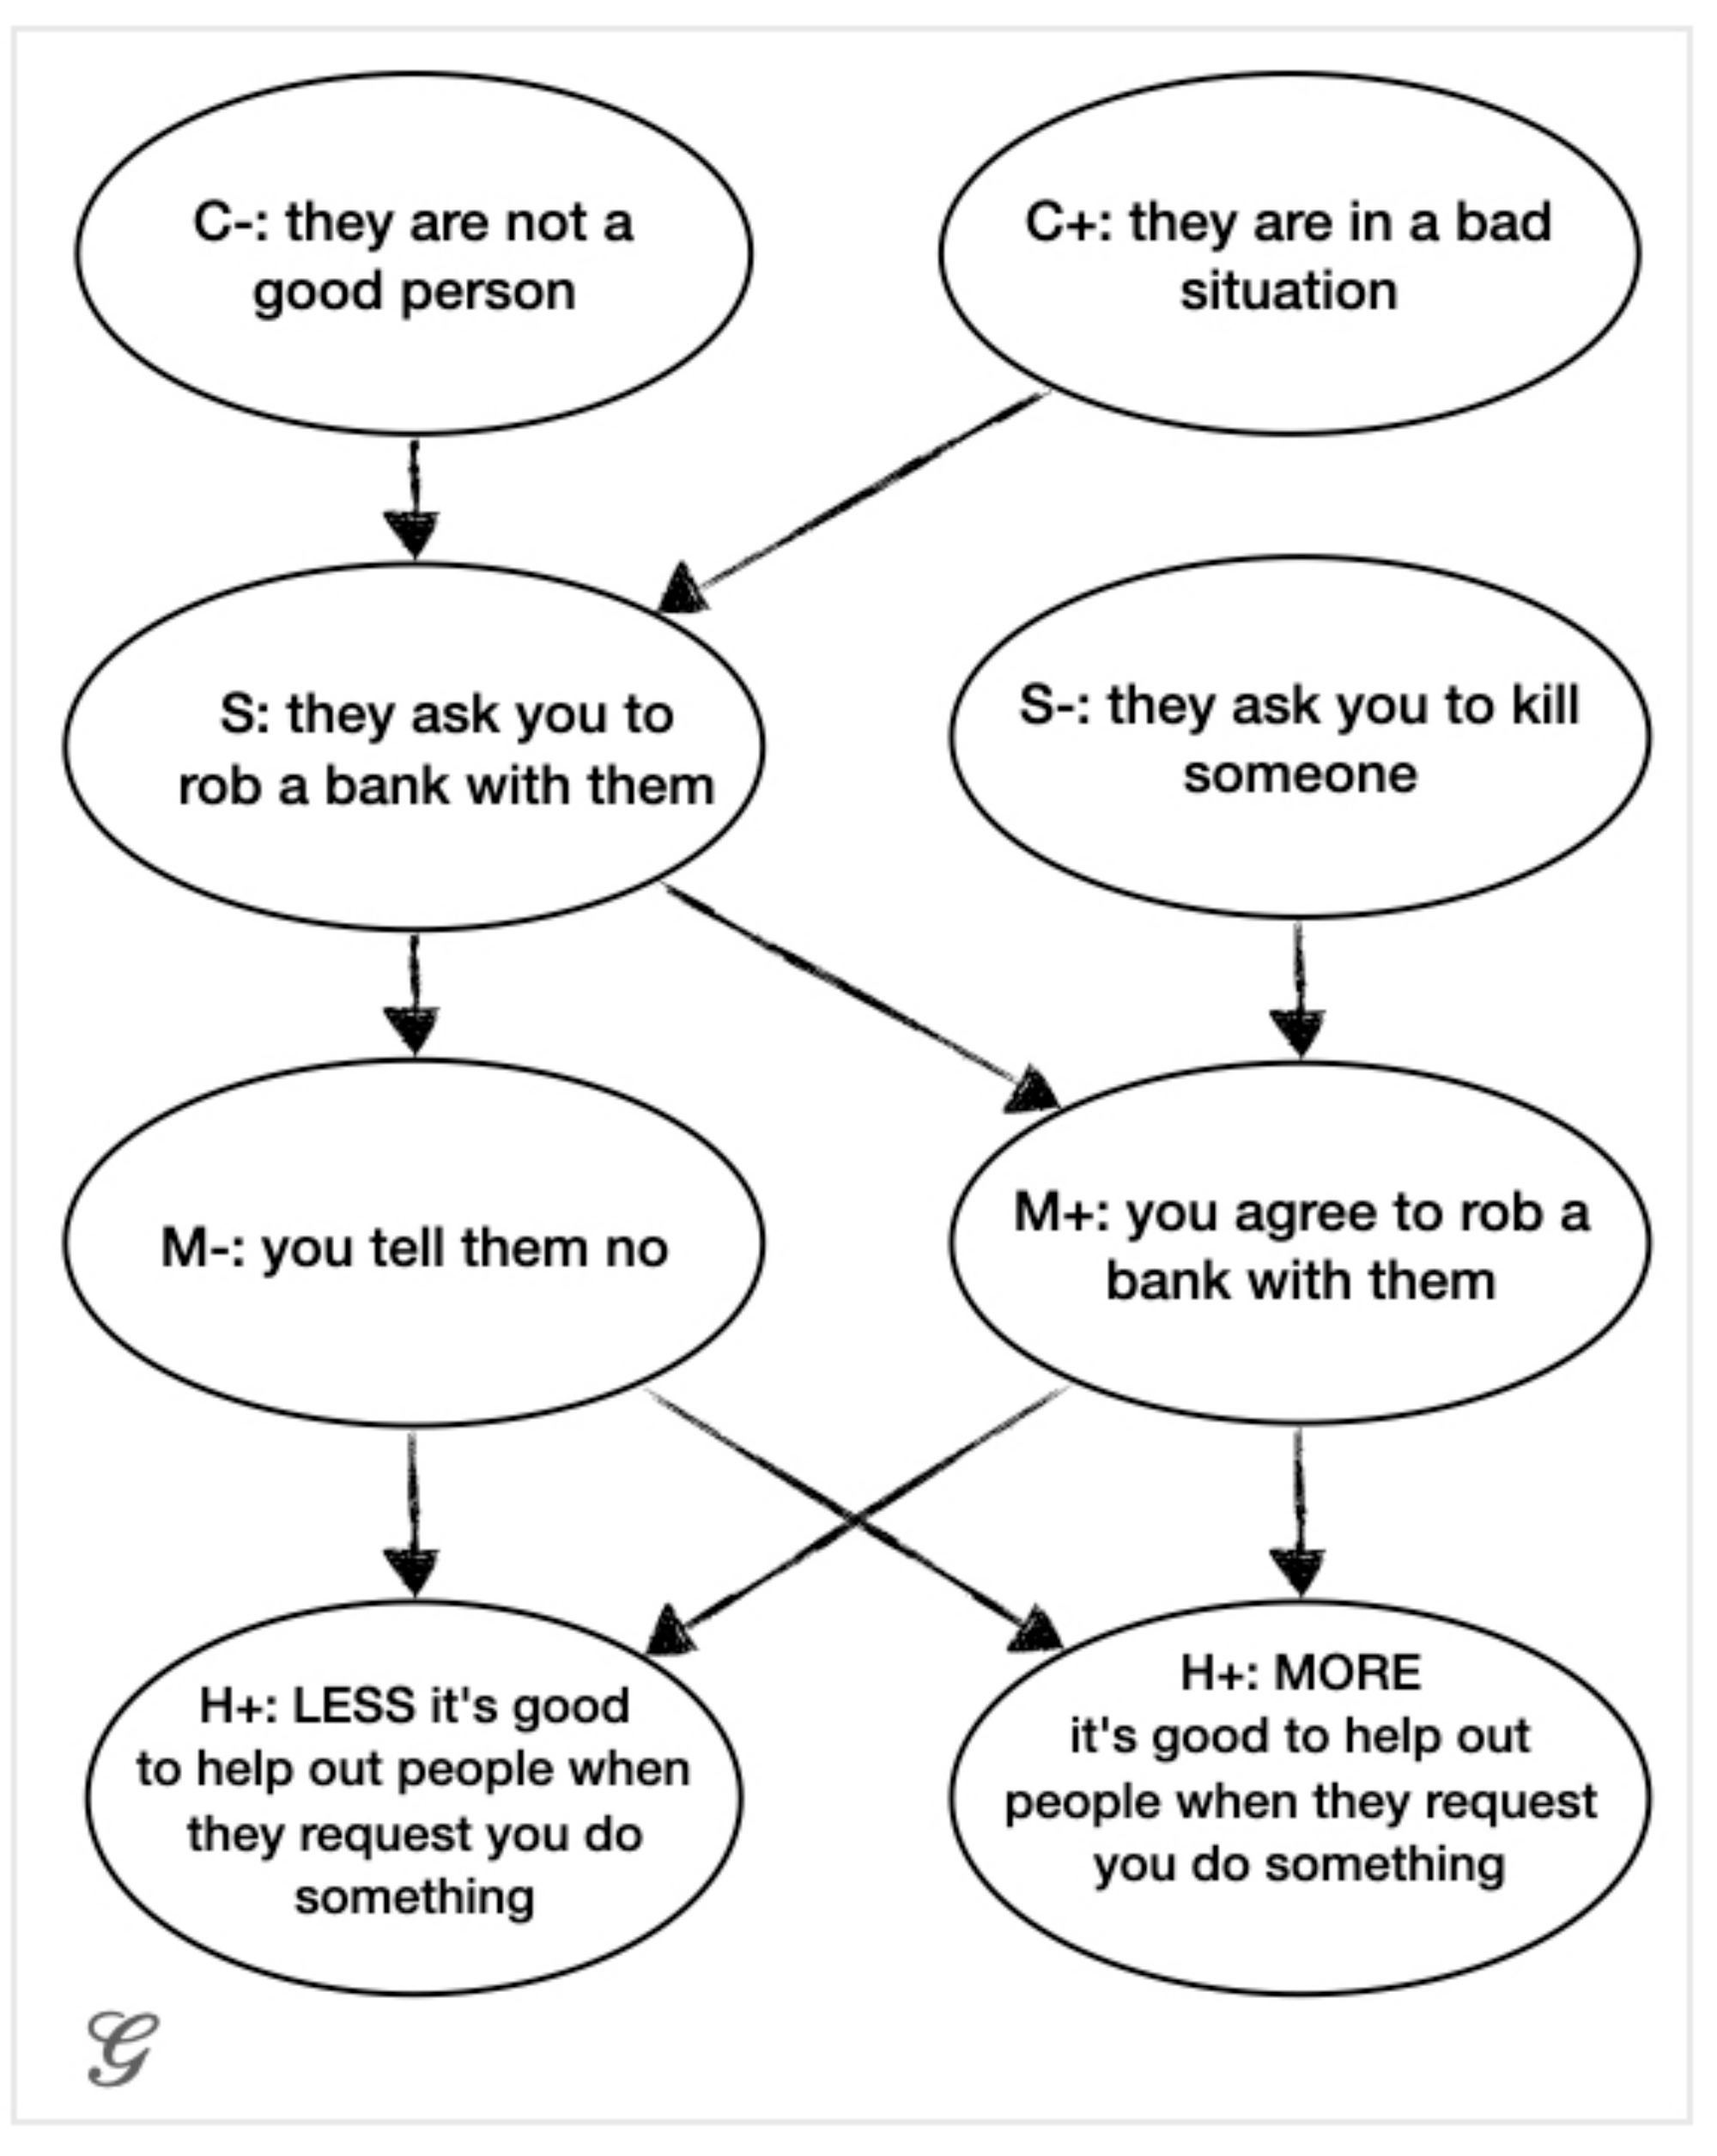}
\end{minipage}
  \captionof{figure}{Incorrect graph generated by \GEN (left) and fixed by \CORR (right) for Defeasible-SNLI dataset. The feedback is `C-, C+ are overlapping, and S, S- are overlapping.'}
  \label{fig:snliexample}
\end{figure*}

\begin{figure*}
\centering
\begin{minipage}{.5\textwidth}
  \centering
  \includegraphics[width=.8\linewidth]{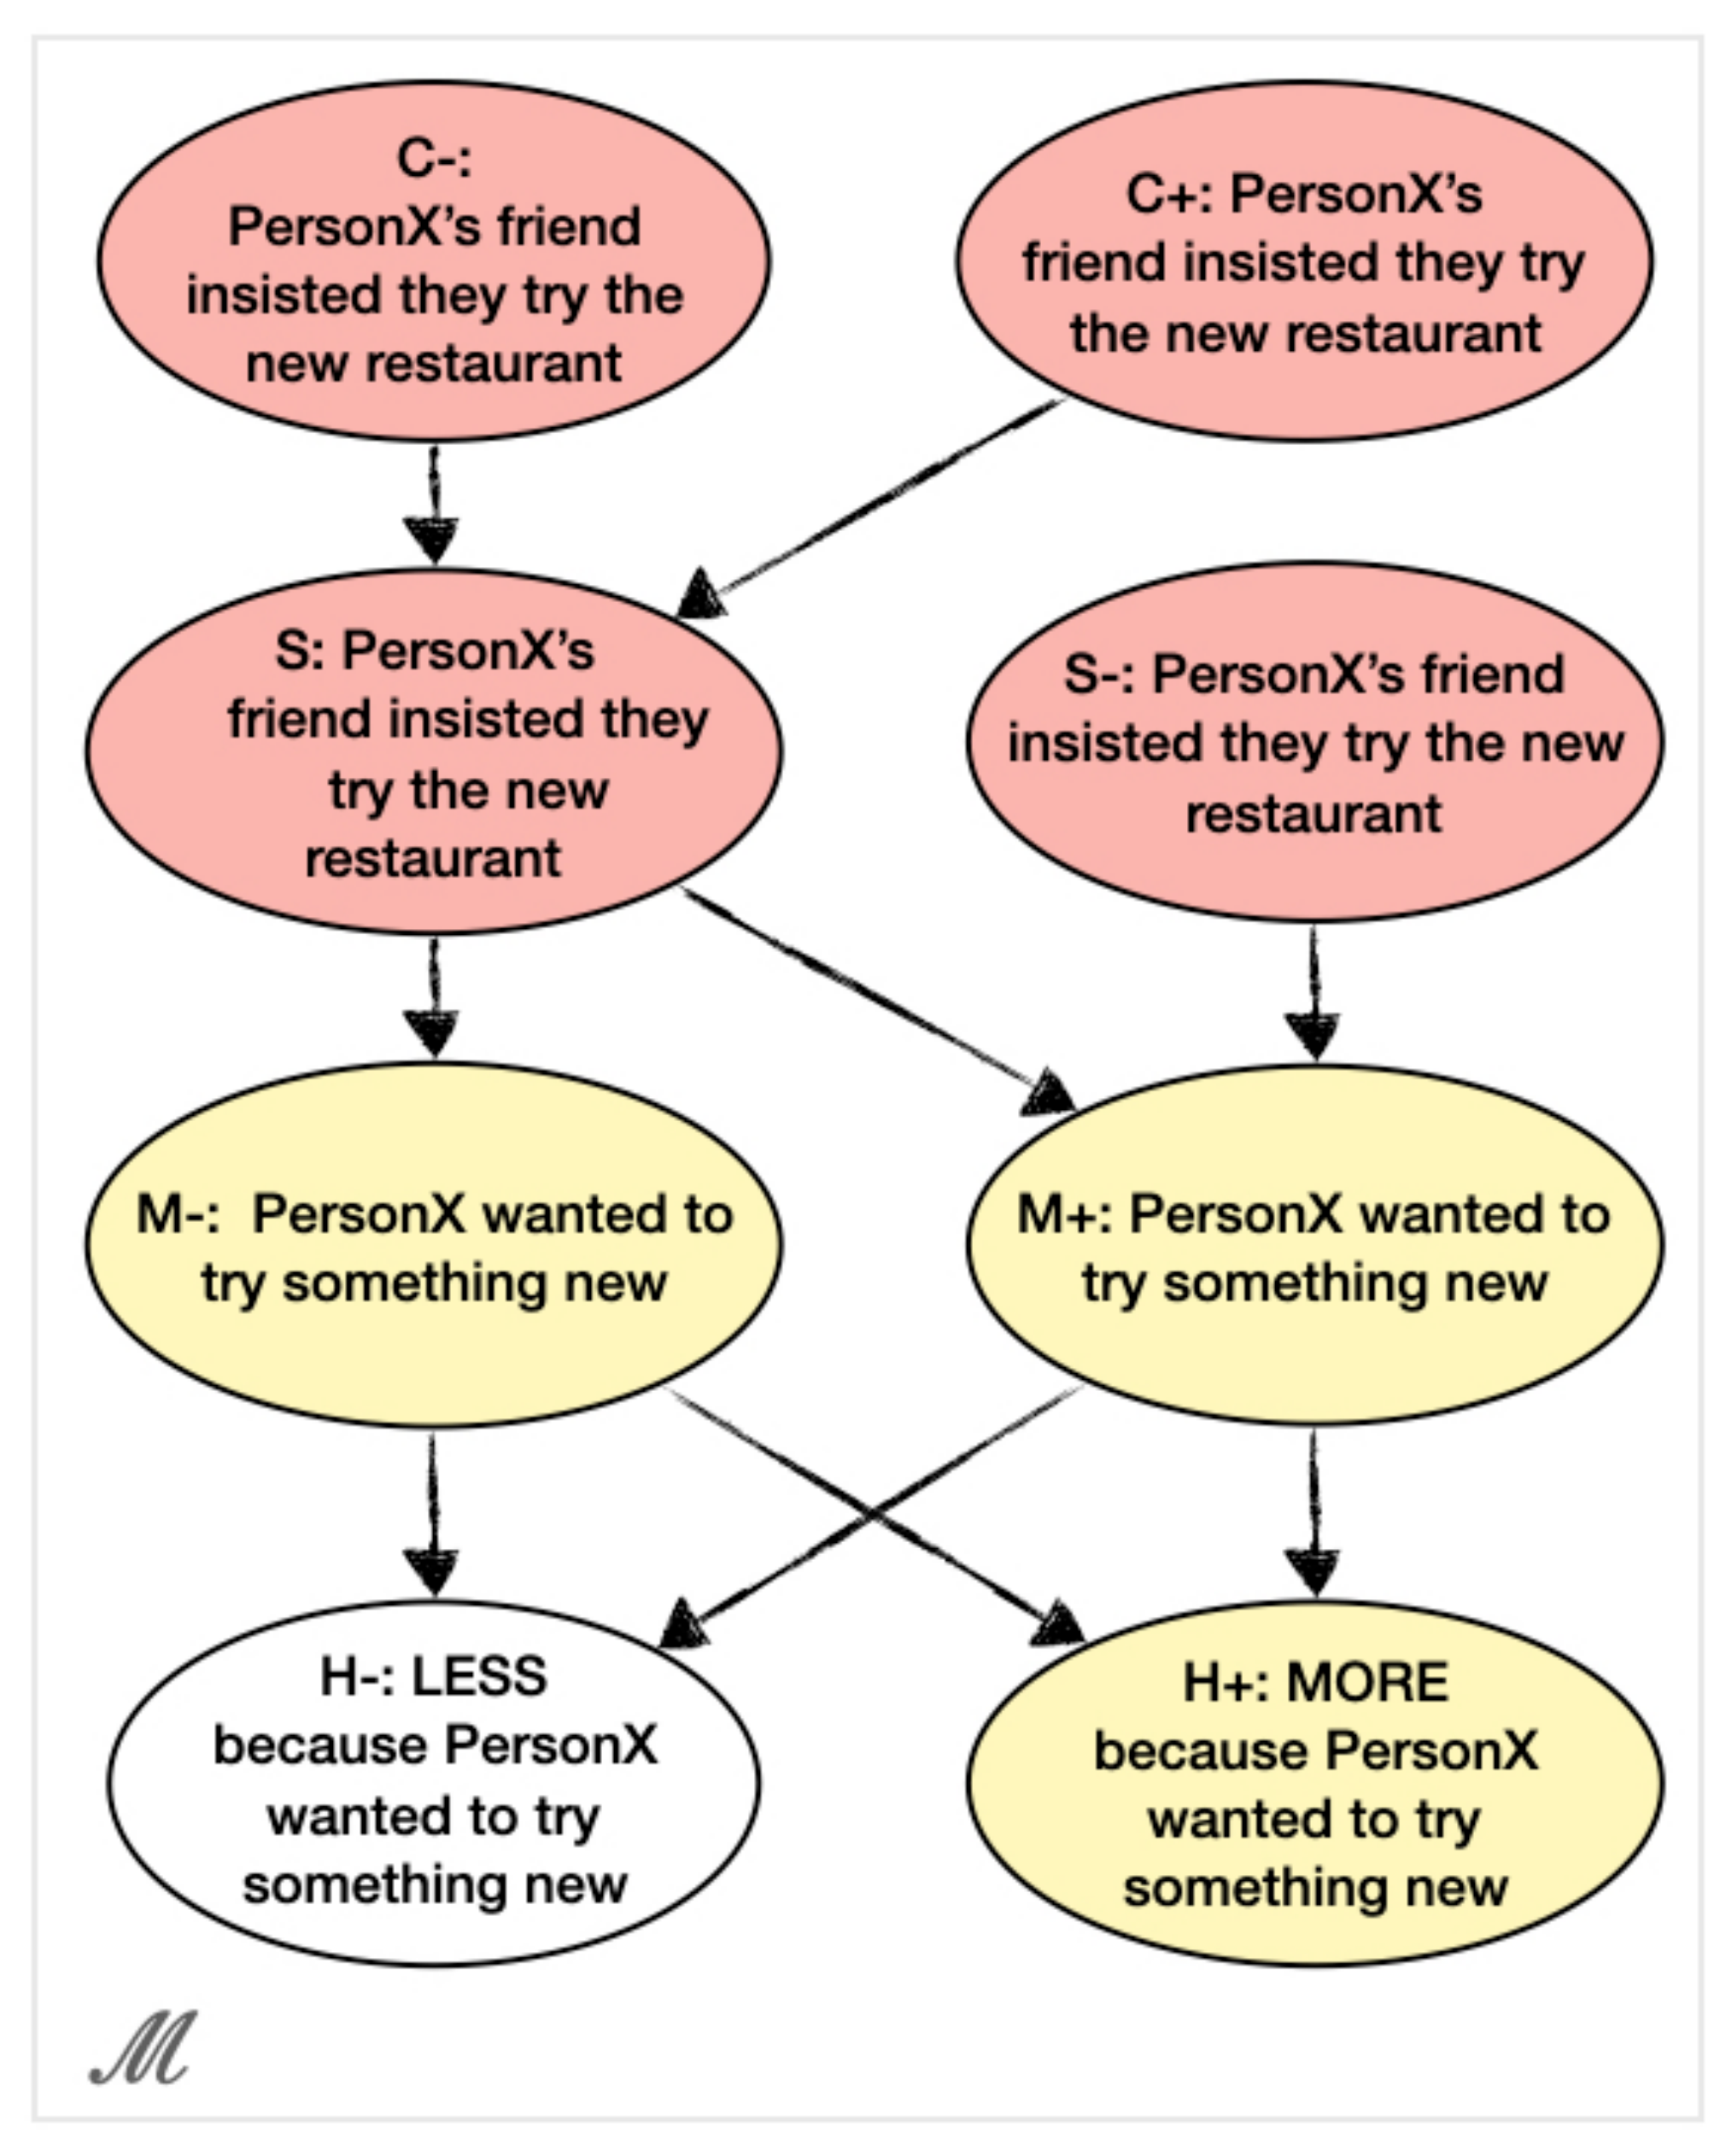}
\end{minipage}%
\begin{minipage}{.5\textwidth}
  \centering
  \includegraphics[width=.8\linewidth]{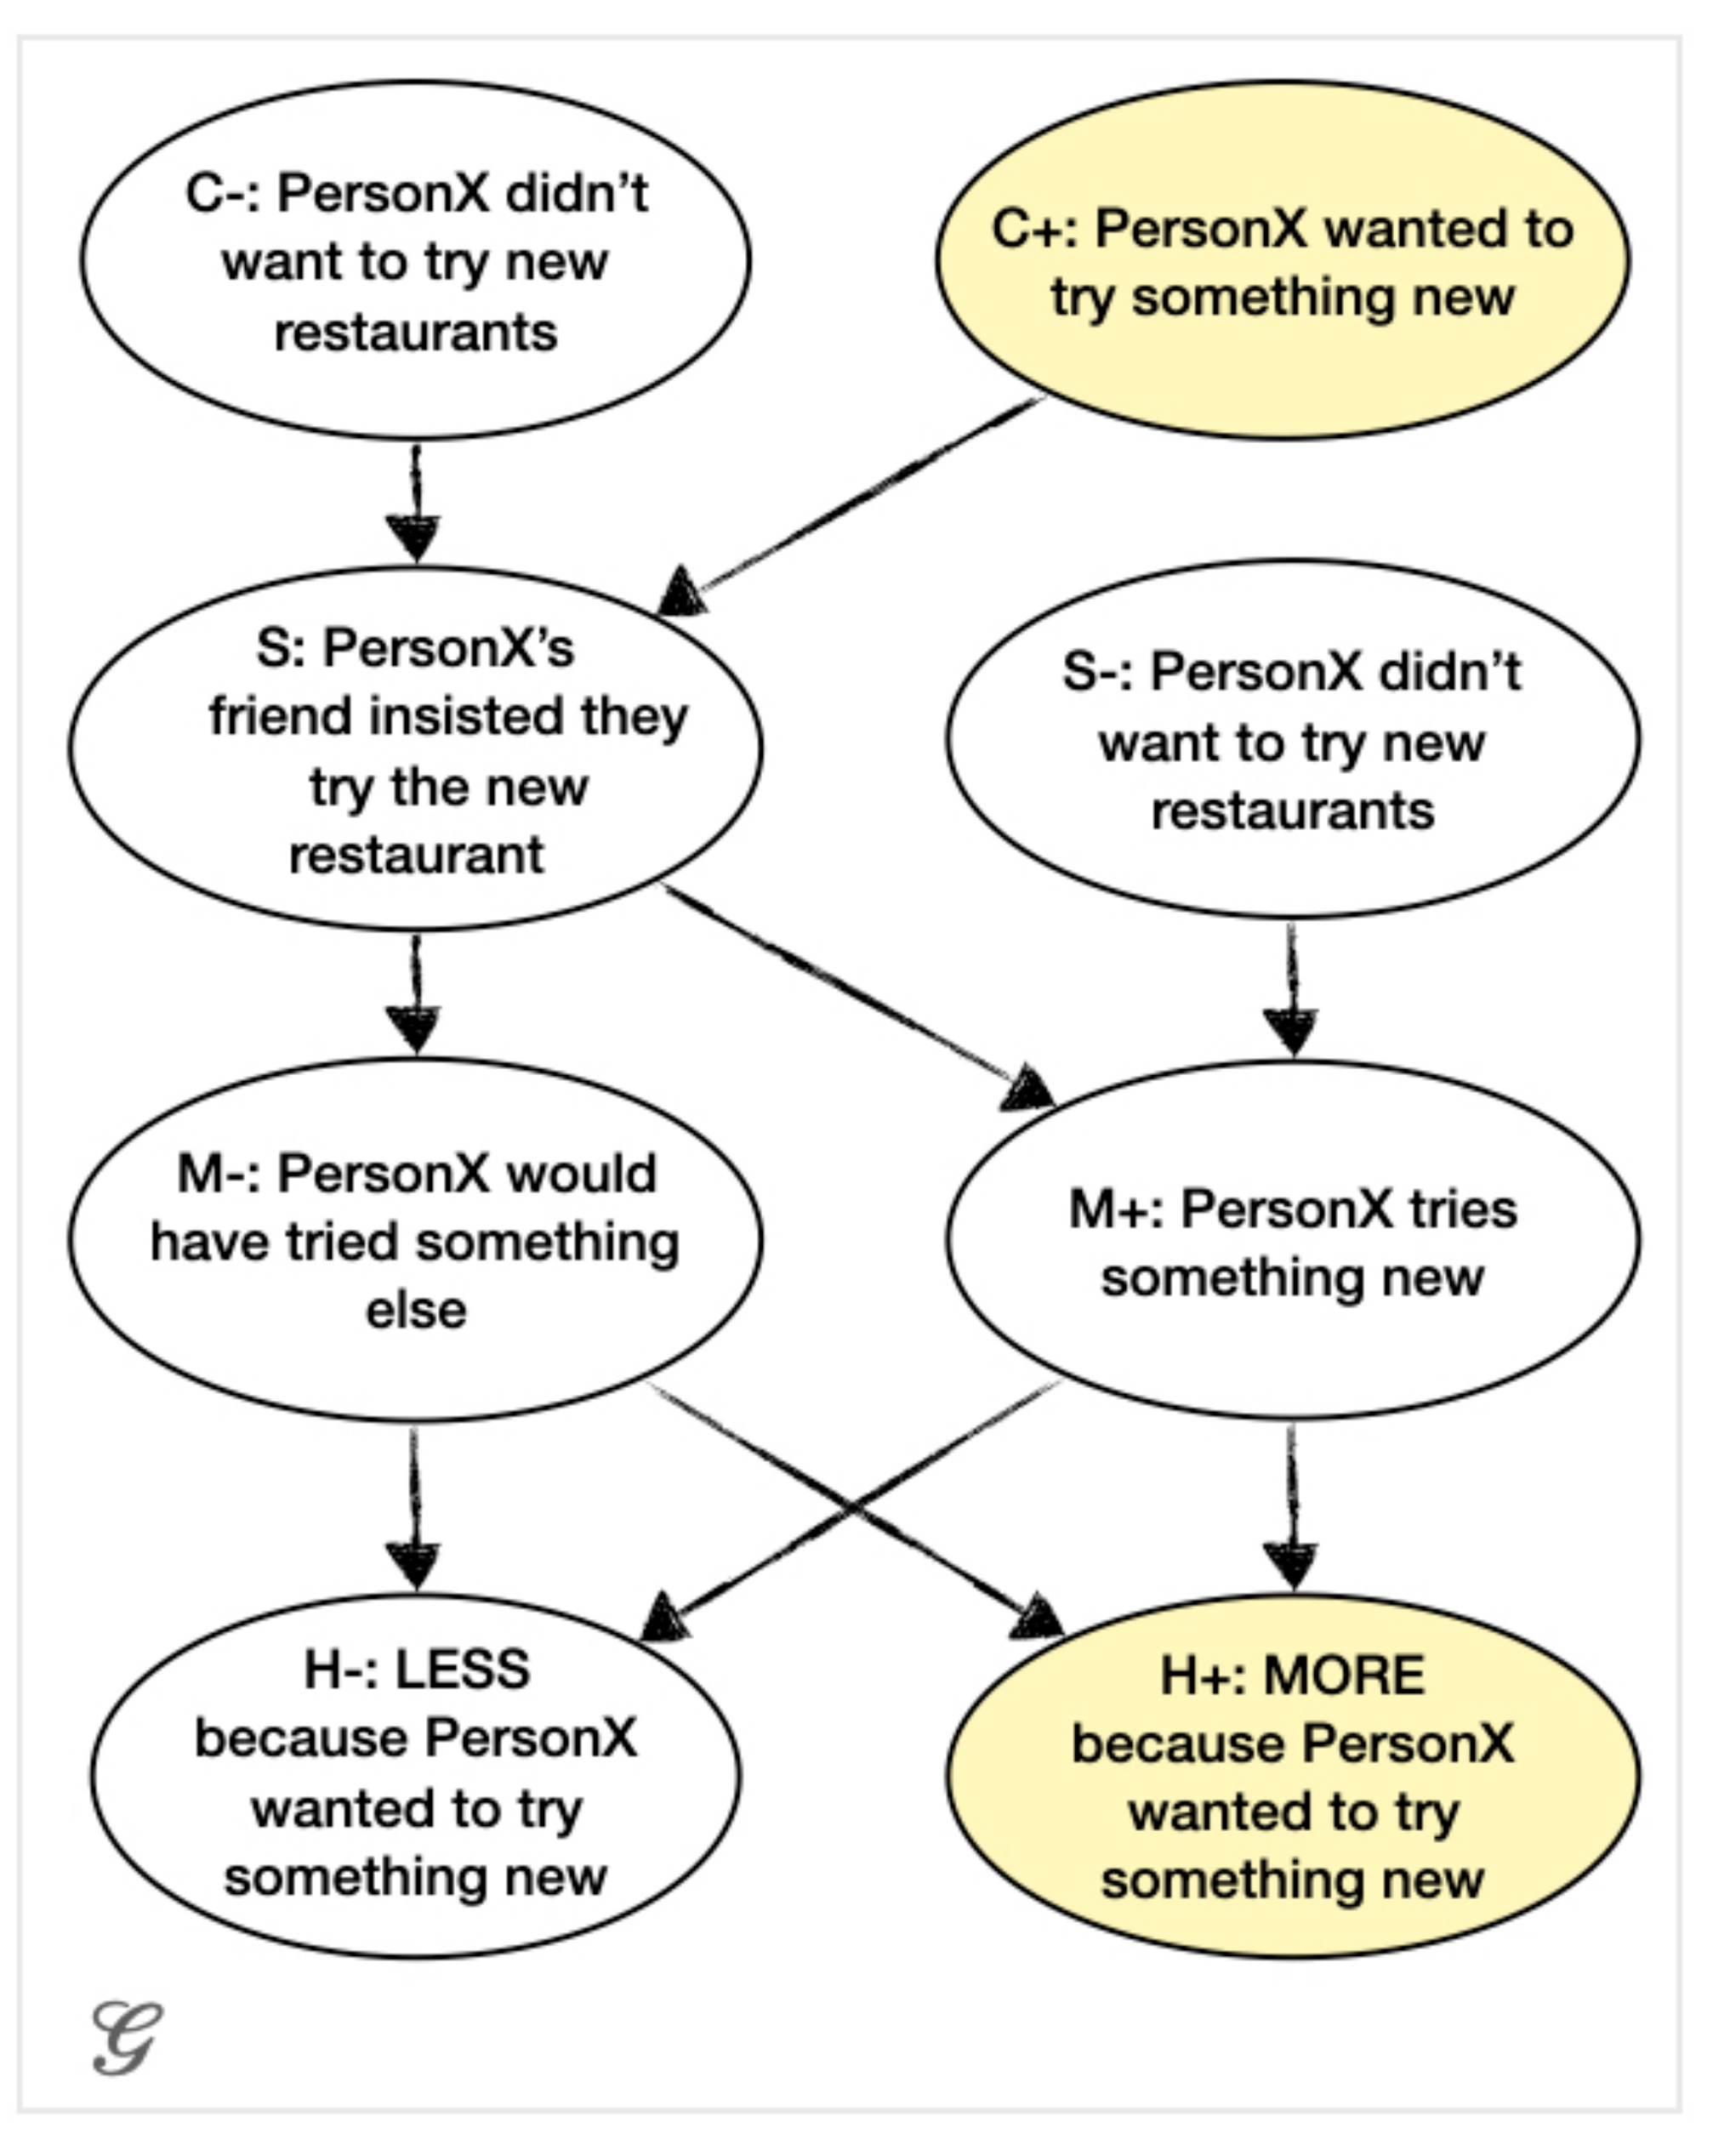}
\end{minipage}
  \captionof{figure}{Incorrect graph generated by \GEN (left) and fixed by \CORR (right) for Defeasible-SOCIAL dataset. The feedback is `C-, C+,S,S- are overlapping, and M-, M+, H+ are overlapping.'}
  \label{fig:socialexample}
\end{figure*}

\begin{figure*}
\centering
\begin{minipage}{.5\textwidth}
  \centering
  \includegraphics[width=.8\linewidth]{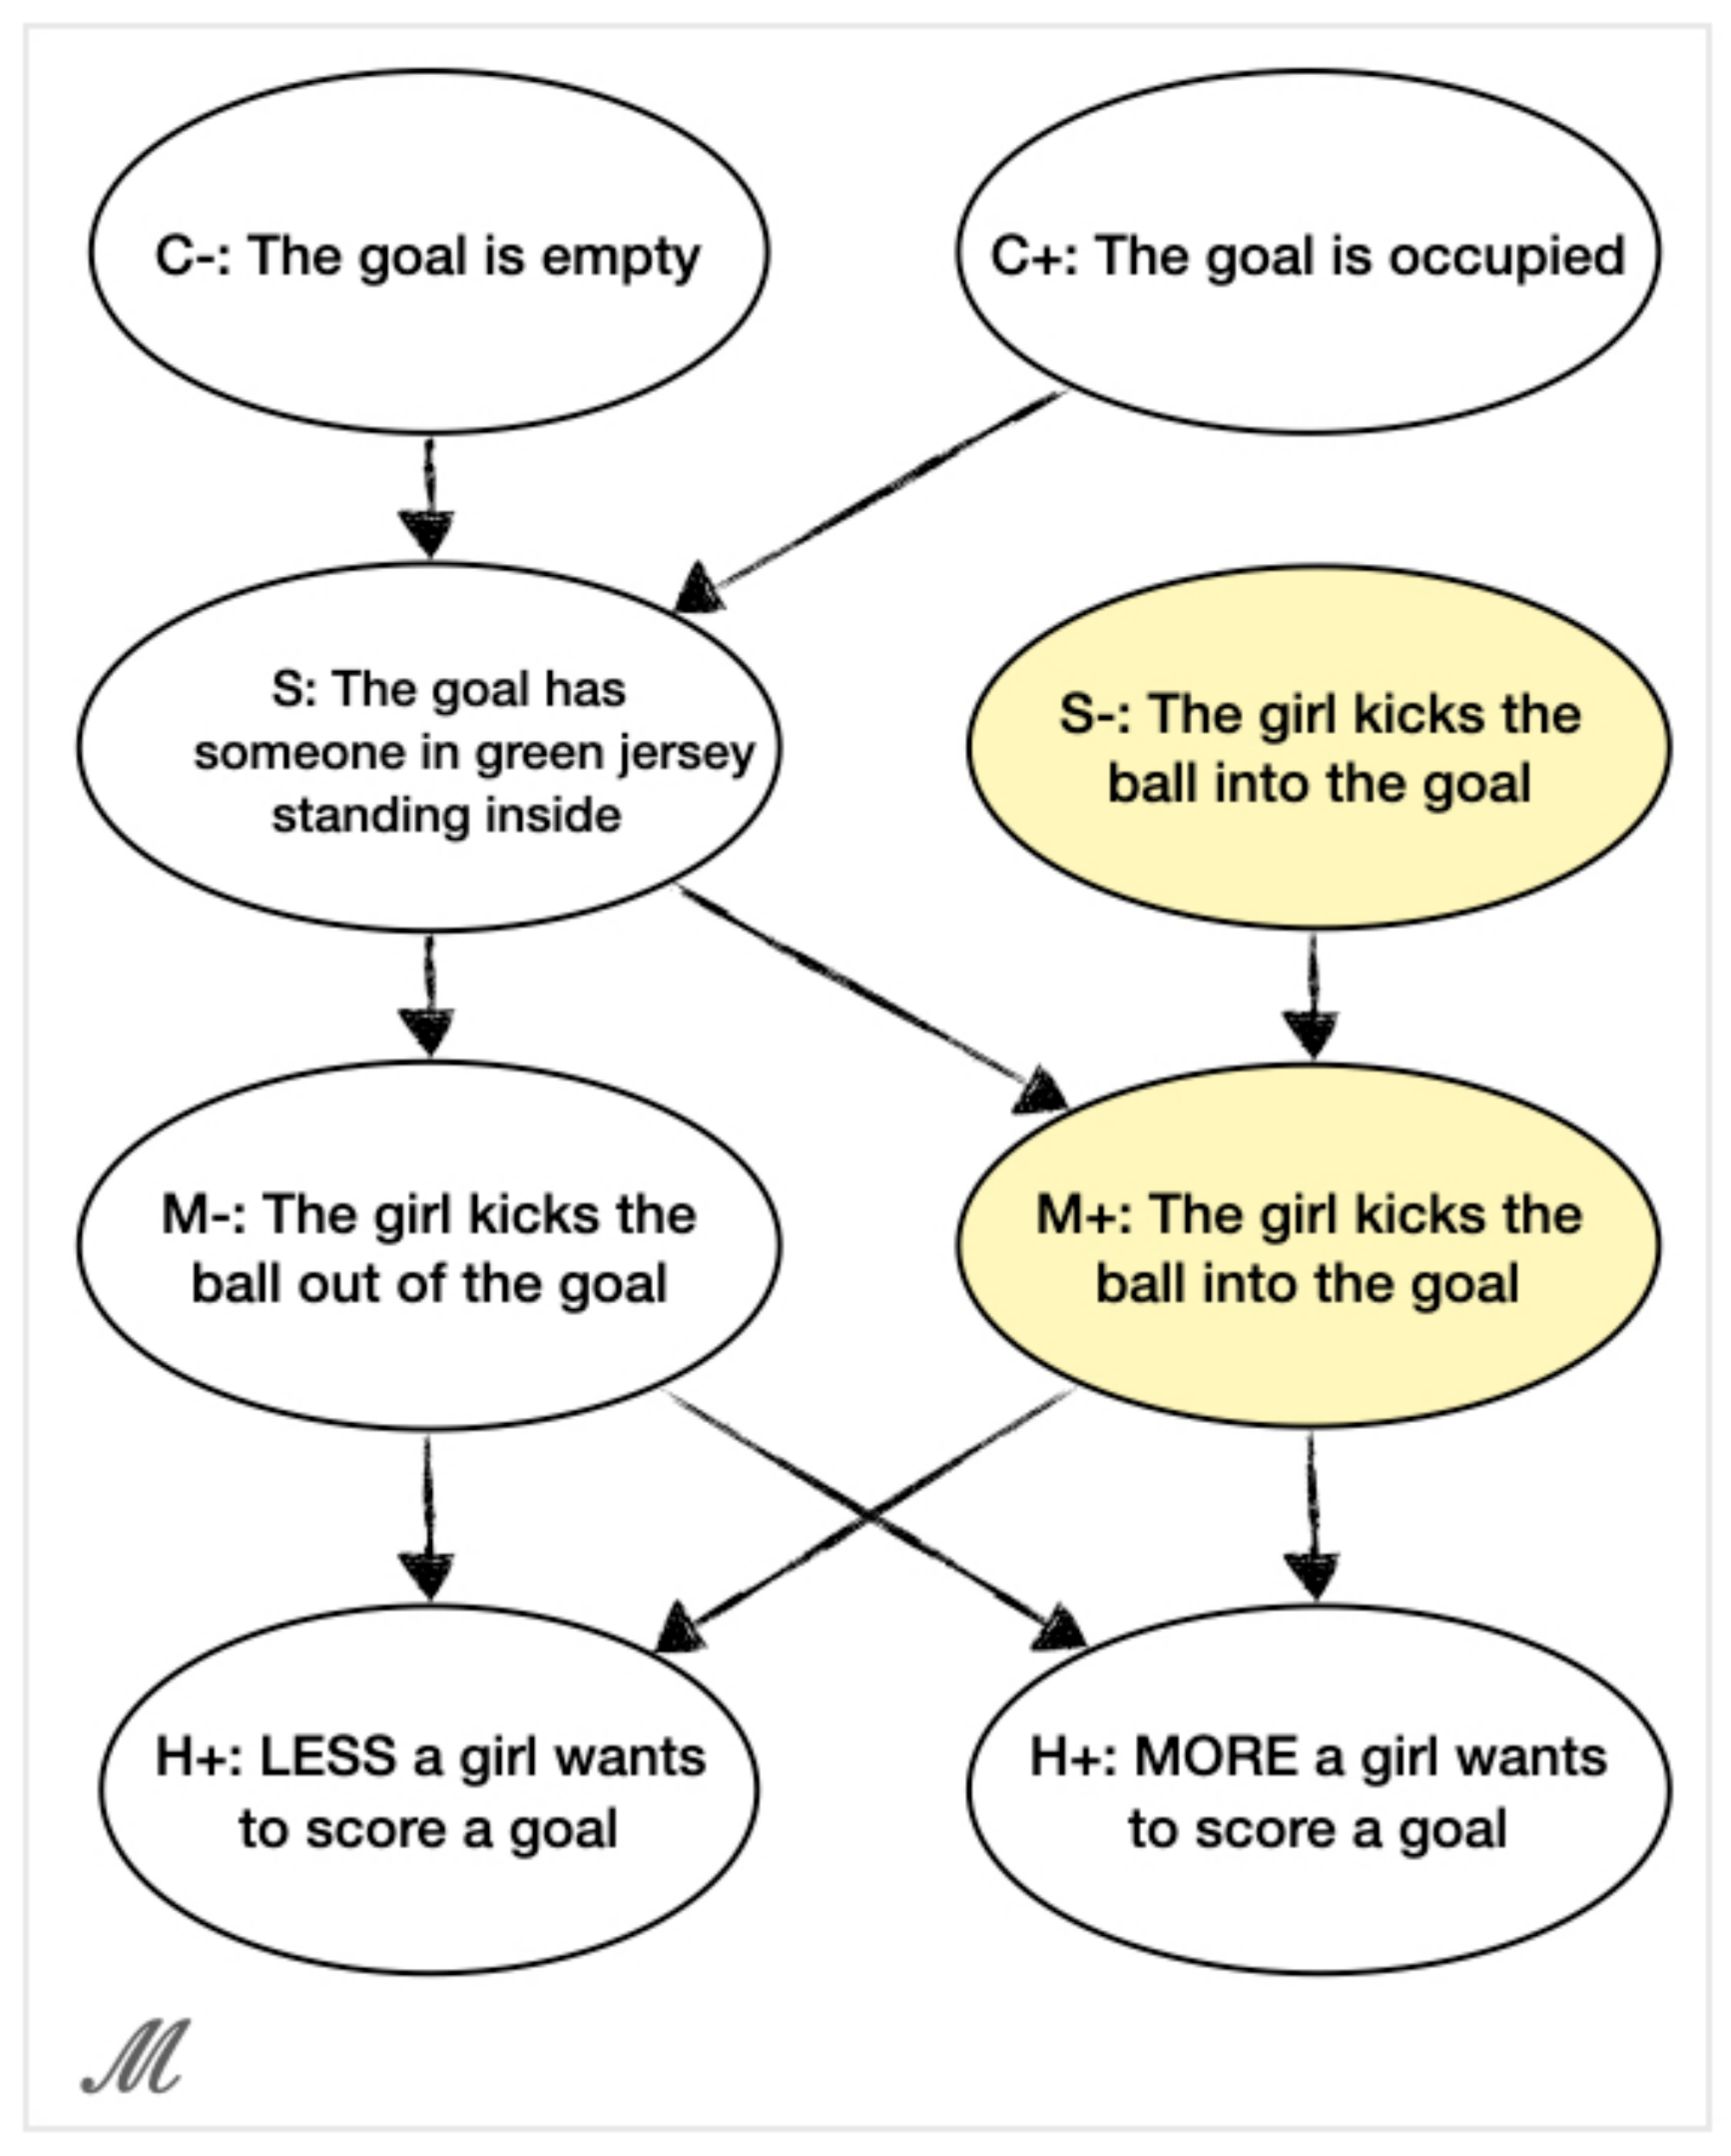}
\end{minipage}%
\begin{minipage}{.5\textwidth}
  \centering
  \includegraphics[width=.8\linewidth]{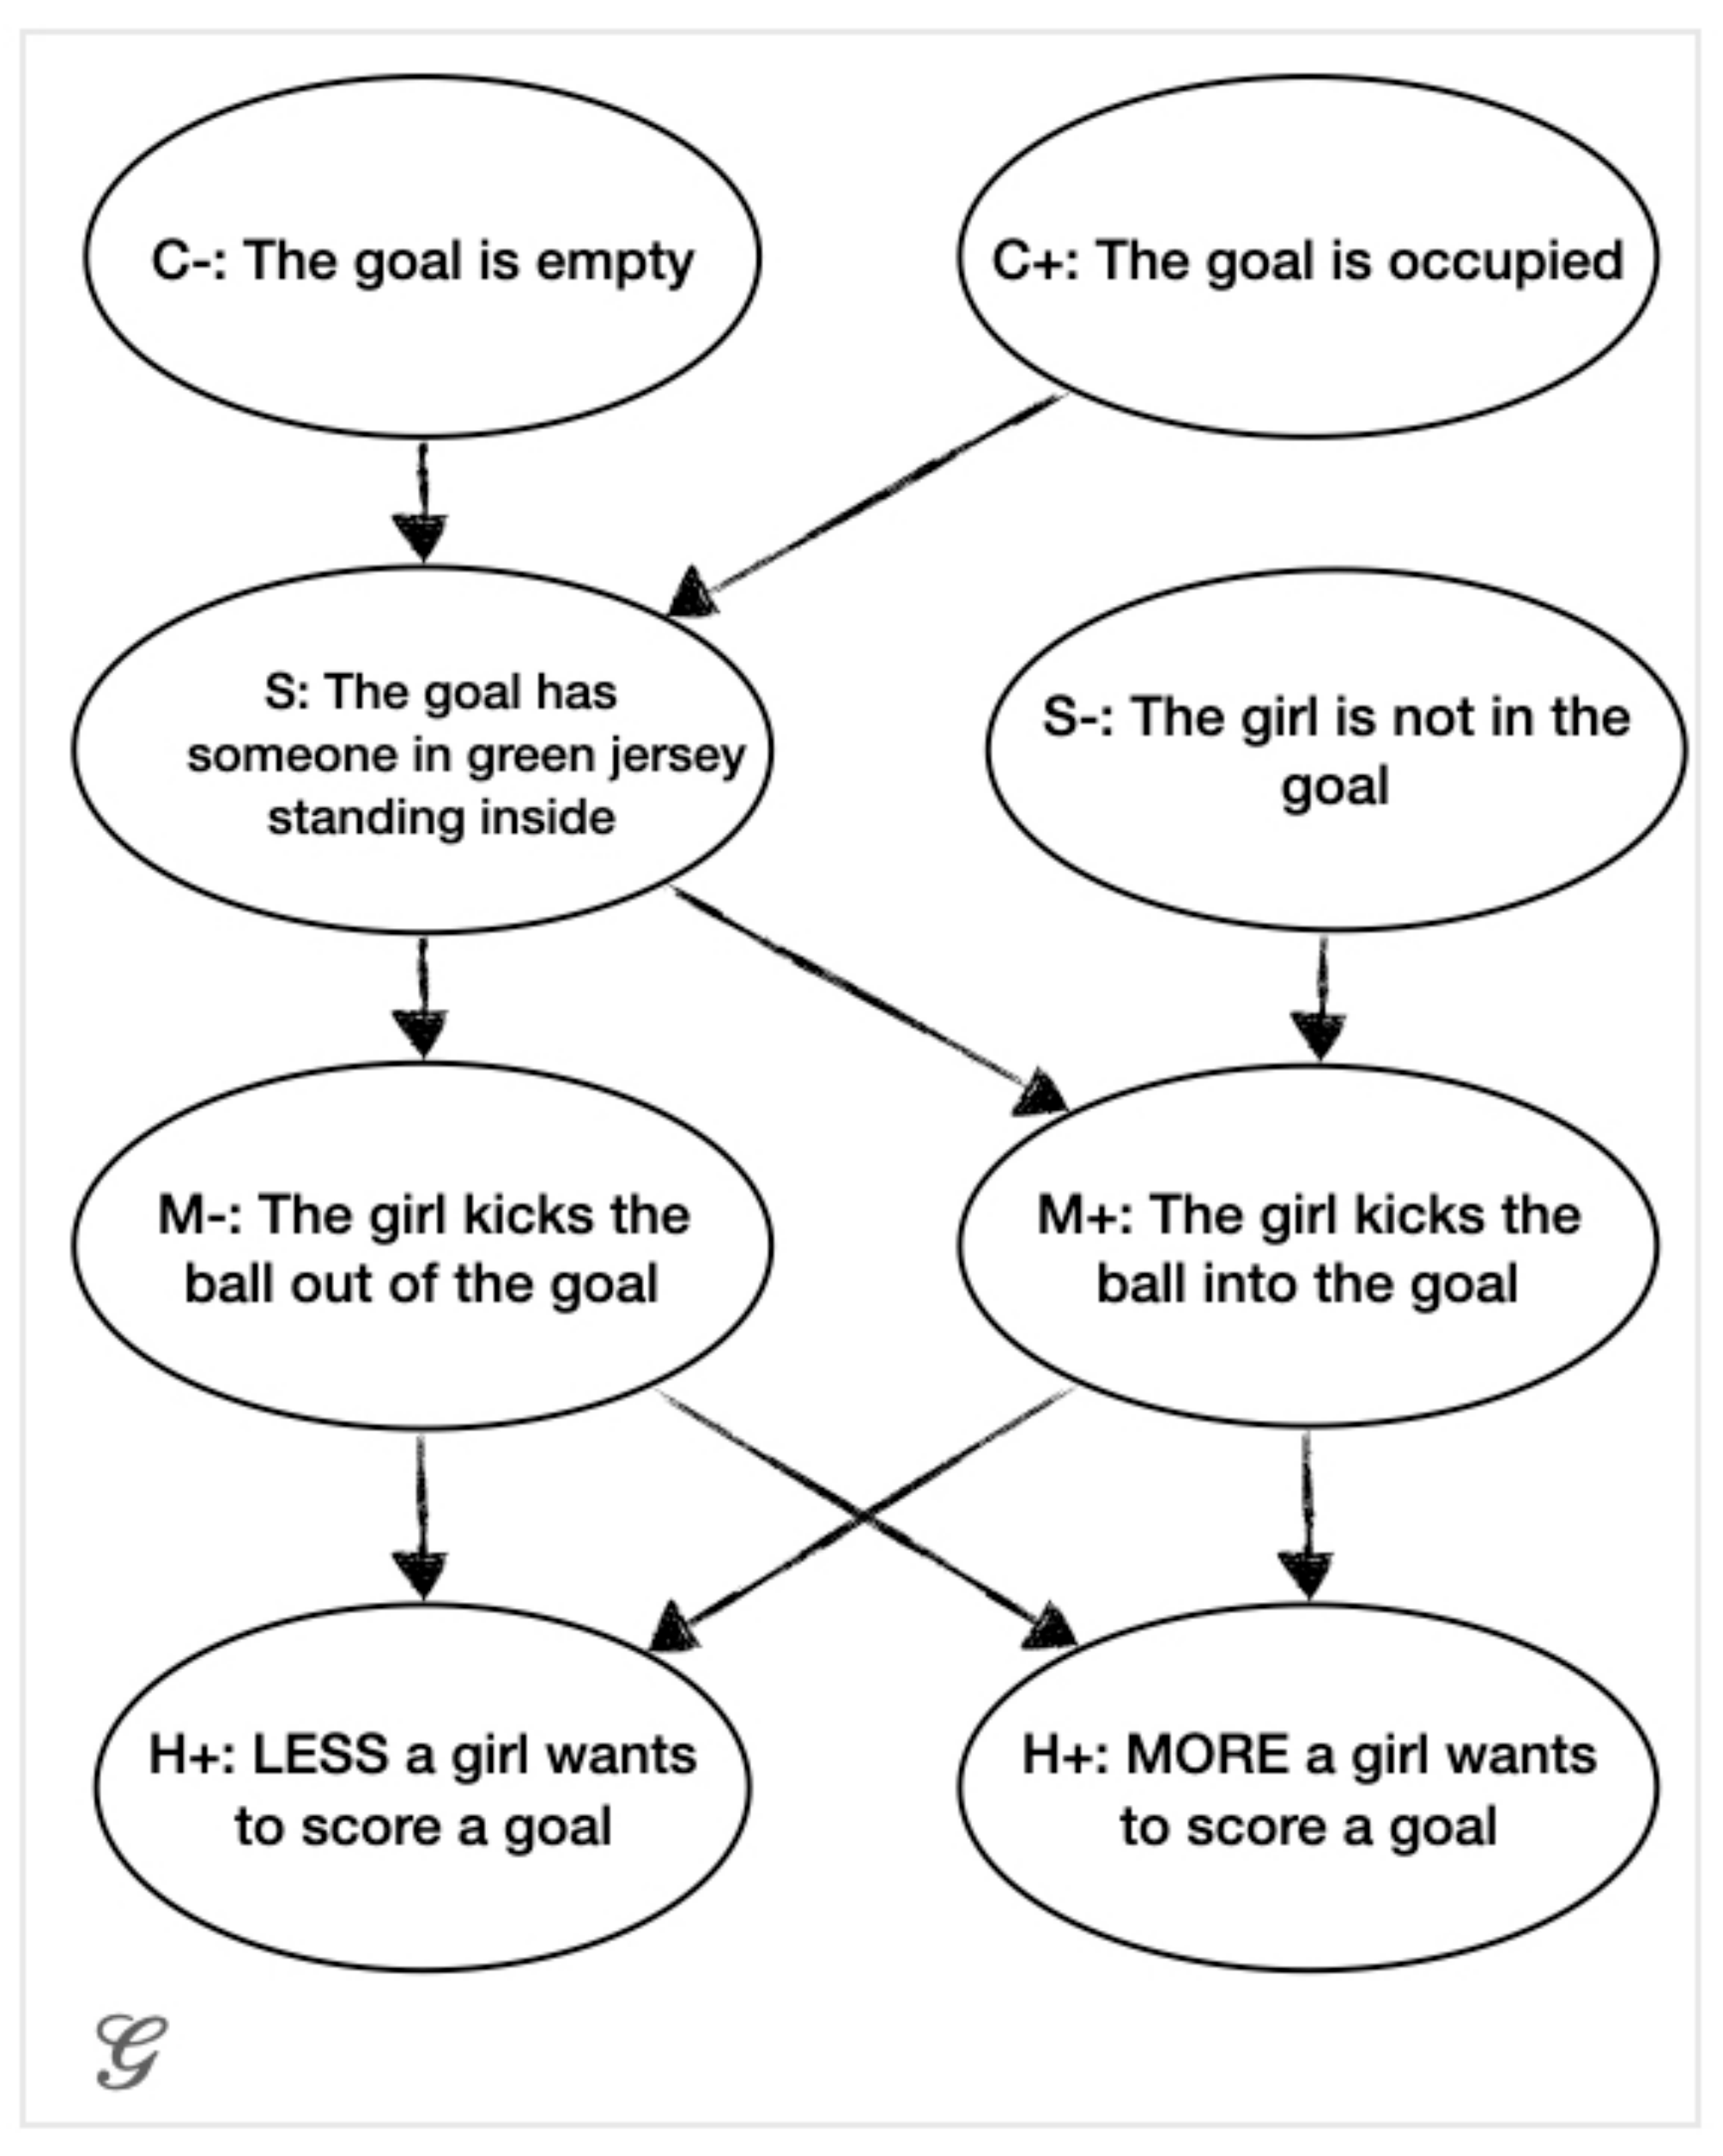}
\end{minipage}
  \captionof{figure}{Incorrect graph generated by \GEN (left) and fixed by \CORR (right) for Defeasible-ATOMIC dataset. The feedback is `S-, M+ are overlapping.;}
  \label{fig:atomicexample}
\end{figure*}
